# Supplementary material for: Static Analysis of Graph Database Transformations
Source: arXiv:2304.05070 source file (2023-04-20)
Supplement: Supplementary file 1 [file appendix.tex]

\section{Appendix}
